# Supplementary material for: High Perceptual Quality Wireless Image Delivery with Denoising Diffusion Models
Source: arXiv:2309.15889 source file (2024-09-20)
Supplement: Supplementary file 1 [file appendix.tex]

\appendix

\begin{figure}
    \centering
    \begin{tabular}[b]{ccc}
   \footnotesize{Original Image} & \footnotesize{DeepJSCC} & \footnotesize{DeepJSCC-Diff (Ours)} \\
    \begin{subfigure}
        \centering    \includegraphics[width=0.28\linewidth]{figures/reconstructed_images/orig_468.png}
    \end{subfigure}&
    \begin{subfigure}
        \centering    \includegraphics[width=0.28\linewidth]{figures/reconstructed_images/468.png}
    \end{subfigure}&
    \begin{subfigure}
        \centering    \includegraphics[width=0.28\linewidth]{figures/reconstructed_images/468_0.png}
    \end{subfigure}\\
    \begin{subfigure}
        \centering    \includegraphics[width=0.28\linewidth]{figures/reconstructed_images/orig_2997.png}
    \end{subfigure}&
    \begin{subfigure}
        \centering    \includegraphics[width=0.28\linewidth]{figures/reconstructed_images/2997.png}
    \end{subfigure}&
    \begin{subfigure}
        \centering    \includegraphics[width=0.28\linewidth]{figures/reconstructed_images/2997_0.png}
    \end{subfigure}\\
    \end{tabular}
    \caption{Qualitative comparison of the reconstructed images from CelebA-HQ dataset for $\rho=0.0052$ and $\mathrm{SNR}_{\mathrm{test}}=1$ \si{\decibel}.}
    \label{fig:reconstructed_images2}
\end{figure}

\Cref{fig:data_transmission} shows the conventional system design for wireless transmission based on separation-based approach. 
\begin{figure}[t!]
\centering
\includegraphics[width=\columnwidth]{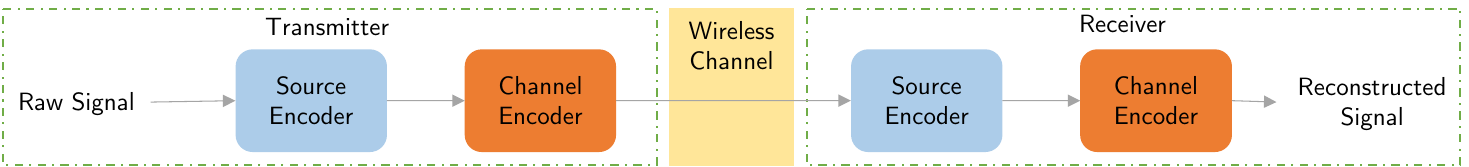}
\vfill
\includegraphics[width=0.75\columnwidth]{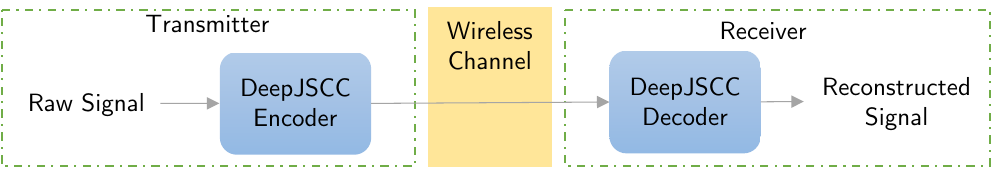}
\caption{Separation-based (top) and \gls{DeepJSCC}-based (bottom) data transmission schemes.}
\label{fig:data_transmission}
\end{figure}

\begin{figure}[!p]
\centering
    \comparisonfig{celeba}{CelebA-HQ}{msssim}{MS-SSIM}{1}
        \caption{\gls{MS-SSIM} comparison of our method with the baselines for $\rho \in \{0.0013,0.0052\}$ over different \glspl{SNR}.}
    \label{fig:comparisons_msssim}
\end{figure}

\begin{figure}
    \centering
    \begin{tabular}[b]{cccc}
\setlength{\tabcolsep}{1pt}   \footnotesize{Original} & \footnotesize{DeepJSCC} & \footnotesize{InverseJSCC} &\footnotesize{Ours} \\
    \begin{subfigure}
        \centering    \includegraphics[width=0.2\columnwidth]{figures/reconstructed_images/new/orig_1225.png}
    \end{subfigure}&
    \begin{subfigure}
        \centering    \includegraphics[width=0.2\columnwidth]{figures/reconstructed_images/new/1225.png}
    \end{subfigure}&
    \begin{subfigure}
        \centering    \includegraphics[width=0.2\columnwidth]{figures/reconstructed_images/new/1225_inversejscc.jpg}
    \end{subfigure}&
    \begin{subfigure}
        \centering    \includegraphics[width=0.2\columnwidth]{figures/reconstructed_images/new/1225_0.png}
    \end{subfigure}\\
    \begin{subfigure}
        \centering    \includegraphics[width=0.2\columnwidth]{figures/reconstructed_images/new/orig_2929.png}
    \end{subfigure}&
    \begin{subfigure}
        \centering    \includegraphics[width=0.2\columnwidth]{figures/reconstructed_images/new/2929.png}
    \end{subfigure}&
    \begin{subfigure}
        \centering    \includegraphics[width=0.2\columnwidth]{figures/reconstructed_images/new/2929_inversejscc.jpg}
    \end{subfigure}&
    \begin{subfigure}
        \centering    \includegraphics[width=0.2\columnwidth]{figures/reconstructed_images/new/2929_0.png}
    \end{subfigure}\\
    \end{tabular}
    \caption{Qualitative comparison of the reconstructed images from CelebA-HQ dataset for $\rho=0.0013$ and $\mathrm{SNR}_{\mathrm{test}}=5$ \si{\decibel}.}
    \label{fig:reconstructed_images3}
\end{figure}
